# Supplementary material for: Exploring Sub-skeleton Trajectories for Interpretable Recognition of Sign Language
Source: arXiv:2202.01390 source file (2022-02-03)
Supplement: Supplementary file 1 [file accuracy_appendix.tex]

\begin{table}[]  %[h!]
\centering
\begin{tabular}{ll|rrrrr}
\hline
\multirow{2}{*}{Classifier} & \multirow{2}{*}{$|C|$} & \multicolumn{5}{c}{Trainers per class}                                        \\
                            &                      & 2             & 3             & 5\%           & 10\%          & 20\%          \\ \hline
\multirow{2}{*}{NN-s}       & reduced              & 79.1          & 83.9          & \textbf{90.1} & \textbf{98.0} & \textbf{99.3} \\
                            & full                 & \textbf{80.2} & \textbf{84.6} & 89.0          & 96.7          & \textbf{99.3} \\ \hline
\multirow{2}{*}{DM-m}       & reduced              & \textbf{80.6} & 89.6          & \textbf{92.2} & 98.4          & \textbf{99.8} \\
                            & full                 & \textbf{80.6} & \textbf{89.7} & 87.7          & \textbf{98.8} & 99.5  \\ \hline      
\end{tabular}
\caption{Comparison of KinTrans accuracy results using a template generated with ($|C|$ is reduced) and without ($|C|$ is full) the feature template mining speed up technique. 
}
\label{tab:accuracy_appendix}
\vspace{-0.35cm}
\end{table}
